# Supplementary material for: GPT-assisted learning of structure-property relationships by graph neural networks: Application to rare-earth doped phosphors
Source: arXiv:2306.14238 ancillary file (2023-12-05)
Supplement: Supplementary file 1 [file suppl.pdf]

**Supplementary Information**

# GPT-assisted learning of structure-property relationships by graph neural networks: Application to rare-earth doped phosphors

Xiang Zhang, Zichun Zhou, Chen Ming, and Yi-Yang Sun

State Key Laboratory of High Performance Ceramics and Superfine Microstructure, Shanghai Institute of Ceramics, Chinese Academy of Sciences, Shanghai 201899, China

The 274 papers used to create the dataset are listed in Table 1. The GPT-parsed and refined dataset of 422 $Eu^{2+}$-activated phosphors, including their host materials' chemical formulas, ICSD collection codes (if available) and emission wavelengths, are listed in Table 2.

HTTP requests were made to OpenAI's Chat Completions API endpoint using OpenAI's Python Library. The full prompt is shown in Table 5.

In Fig. 3e in the main text, we inspected the GPT-n series of models' performance by analyzing their parsing result on Ref. [1], shown in Table 3.

When matching the 422 GPT-parsed chemical formulas to the ICSD database, rarely multiple matches are found (Fig. 1). Most of the time, the multiple matches are but duplicates, essentially identical crystal structure with slight numerical deviations. These cases can be identified by creating a list of bijective atomic distances (bond lengths) for each crystal structure, and comparing their distributions as a fingerprint. Such comparisons for all cases of 2 ICSD matches are shown in Fig. 4. Fingerprinting crystal structures for comparison is a non-trivial topic in itself[2, 3], which we do not delve deeply into here.

We used Ref. [4]'s original CGCNN implementation in PyTorch (Fig. 6). The default neural network architecture of 64 hidden atom features, 3 convolutional layers, 128 hidden features after pooling, and 1 hidden layer after pooling were found to be optimal. The typical learning curve is shown in Fig. 5. Incidentally, we noticed that it would be possible to overfit to sub-1Å accuracy if we were to remove all of Ref. [5]'s contributions from the dataset.

In Table 1 in the main text, we compared different CGCNN setups and their performance on the 264-phosphor dataset in terms of a 10-fold-averaged $R^2$ score. The original data is shown in Table 4.

In Fig. 4b in the main text, we plotted the mapping from chemical formulas (or their 2D embeddings) to emission wavelengths as a color map. The 2D embedding is created as follows. Each element is represented by its period and group numbers and one-hot encoded, creating two vectors of length 7 and 18, which are concatenated. For each chemical formula, the one-hot elemental representations for all constituent atoms are added together and normalized, creating a multi-hot vector of length 25 where each element represents the mole fraction of the corresponding element. The multi-hot vectors are then embedded into the 2D space using UMAP[6], a library capable of unsupervised and supervised dimensionality reduction. Finally, the emission wavelengths are mapped to real-life RGB colors, and a 2D scatter plot with a color map created.

Supplementary Table 1: DOIs of articles in dataset

| DOI |
| --- |
| **Reviews** |
| 10.1002/adom.202102287 |
| 10.1007/s10853-009-3668-4 |
| 10.1016/S0022-2313(03)00078-4 |
| 10.1016/j.jre.2019.10.005 |
| 10.1021/acs.chemrev.7b00284 |
| 10.1021/acs.jpclett.0c01471 |
| 10.1039/C3CS60314H |
| 10.3390/ma3042536 |
| 10.1016/B978-0-08-101942-9.00005-8 |
| 10.1146/annurev-matsci-073012-125702 |
| 10.1016/j.jlumin.2018.09.047 |
| **Articles** |
| 10.1002/9783527621064.ch3 |
| 10.1002/ZAAC.200870072 |
| 10.1002/adma.201003640 |
| 10.1002/adma.201802489 |
| 10.1002/adom.201500078 |
| 10.1002/adom.201901859 |
| 10.1002/anie.201905787 |
| 10.1002/chem.201000660 |
| 10.1002/chem.201201953 |
| 10.1002/chem.201500047 |
| 10.1002/zaac.201400487 |
| 10.1007/s00340-012-4969-x |
| 10.1007/s10853-005-1237-z |
| 10.1007/s10853-008-2764-1 |
| 10.1007/s10854-007-9466-3 |
| 10.1007/s10854-019-00995-w |
| 10.1007/s11801-013-3008-4 |
| 10.1016/0022-4596(89)90181-3 |

| DOI (continued) |
| --- |
| 10.1016/0022-4596(91)90365-O |
| 10.1016/0254-0584(93)90080-6 |
| 10.1016/0925-8388(93)90143-B |
| 10.1016/S0167-577X(02)00567-0 |
| 10.1016/S0925-8388(97)00550-1 |
| 10.1016/S1002-0721(14)60426-9 |
| 10.1016/S1002-0721(14)60441-5 |
| 10.1016/S1002-0721(14)60490-7 |
| 10.1016/S1002-0721(14)60574-3 |
| 10.1016/j.cej.2016.10.109 |
| 10.1016/j.cej.2019.122528 |
| 10.1016/j.cej.2019.124004 |
| 10.1016/j.ceramint.2013.03.068 |
| 10.1016/j.ceramint.2013.04.097 |
| 10.1016/j.ceramint.2015.07.193 |
| 10.1016/j.ceramint.2015.11.157 |
| 10.1016/j.ceramint.2016.03.216 |
| 10.1016/j.ceramint.2016.04.182 |
| 10.1016/j.ceramint.2017.03.142 |
| 10.1016/j.ceramint.2017.12.082 |
| 10.1016/j.ceramint.2018.08.076 |
| 10.1016/j.cplett.2007.05.023 |
| 10.1016/j.cplett.2016.01.068 |
| 10.1016/j.cplett.2021.138516 |
| 10.1016/j.ijleo.2015.05.003 |
| 10.1016/j.jallcom.2004.04.134 |
| 10.1016/j.jallcom.2005.09.041 |
| 10.1016/j.jallcom.2006.06.103 |
| 10.1016/j.jallcom.2010.09.094 |
| 10.1016/j.jallcom.2011.10.065 |
| 10.1016/j.jallcom.2013.05.188 |
| 10.1016/j.jallcom.2015.01.069 |
| 10.1016/j.jallcom.2015.05.280 |
| 10.1016/j.jallcom.2016.02.100 |
| 10.1016/j.jallcom.2017.10.022 |

| DOI (continued) |
|---|
| 10.1016/j.jallcom.2019.151956 |
| 10.1016/j.jallcom.2020.155469 |
| 10.1016/j.jallcom.2021.158634 |
| 10.1016/j.jallcom.2022.165092 |
| 10.1016/j.jeurceramsoc.2019.10.022 |
| 10.1016/j.jlumin.2006.01.112 |
| 10.1016/j.jlumin.2006.01.171 |
| 10.1016/j.jlumin.2009.07.006 |
| 10.1016/j.jlumin.2009.10.030 |
| 10.1016/j.jlumin.2011.06.004 |
| 10.1016/j.jlumin.2012.05.004 |
| 10.1016/j.jlumin.2012.11.012 |
| 10.1016/j.jlumin.2013.02.012 |
| 10.1016/j.jlumin.2013.09.037 |
| 10.1016/j.jlumin.2013.09.041 |
| 10.1016/j.jlumin.2013.09.047 |
| 10.1016/j.jlumin.2013.10.003 |
| 10.1016/j.jlumin.2013.10.017 |
| 10.1016/j.jlumin.2013.11.083 |
| 10.1016/j.jlumin.2016.07.015 |
| 10.1016/j.jlumin.2016.11.013 |
| 10.1016/j.jlumin.2017.01.004 |
| 10.1016/j.jlumin.2017.06.009 |
| 10.1016/j.jlumin.2018.07.002 |
| 10.1016/j.jlumin.2018.08.044 |
| 10.1016/j.jlumin.2020.117544 |
| 10.1016/j.jlumin.2020.117786 |
| 10.1016/j.joule.2018.01.012 |
| 10.1016/j.jssc.2004.07.054 |
| 10.1016/j.jssc.2008.04.017 |
| 10.1016/j.jssc.2008.10.031 |
| 10.1016/j.jssc.2017.07.026 |
| 10.1016/j.materresbull.2013.01.042 |
| 10.1016/j.materresbull.2013.05.122 |
| 10.1016/j.materresbull.2013.08.011 |

| DOI (continued) |
|---|
| 10.1016/j.materresbull.2013.09.035 |
| 10.1016/j.materresbull.2013.09.054 |
| 10.1016/j.materresbull.2013.11.012 |
| 10.1016/j.materresbull.2013.11.049 |
| 10.1016/j.materresbull.2014.12.044 |
| 10.1016/j.materresbull.2014.12.051 |
| 10.1016/j.materresbull.2015.06.009 |
| 10.1016/j.materresbull.2017.05.005 |
| 10.1016/j.materresbull.2018.07.036 |
| 10.1016/j.matlet.2006.07.149 |
| 10.1016/j.matlet.2007.04.042 |
| 10.1016/j.matlet.2007.10.030 |
| 10.1016/j.matlet.2011.07.050 |
| 10.1016/j.matlet.2012.02.095 |
| 10.1016/j.mseb.2007.07.042 |
| 10.1016/j.mseb.2014.10.012 |
| 10.1016/j.optcom.2011.05.022 |
| 10.1016/j.optlastec.2016.04.010 |
| 10.1016/j.optmat.2007.01.008 |
| 10.1016/j.optmat.2010.11.023 |
| 10.1016/j.optmat.2011.07.003 |
| 10.1016/j.optmat.2011.10.004 |
| 10.1016/j.optmat.2012.01.034 |
| 10.1016/j.optmat.2012.11.016 |
| 10.1016/j.optmat.2013.05.030 |
| 10.1016/j.optmat.2014.02.024 |
| 10.1016/j.optmat.2014.10.003 |
| 10.1016/j.optmat.2014.12.042 |
| 10.1016/j.optmat.2016.02.026 |
| 10.1016/j.optmat.2016.05.048 |
| 10.1016/j.optmat.2017.01.033 |
| 10.1016/j.optmat.2017.06.012 |
| 10.1016/j.physb.2010.10.059 |
| 10.1016/j.poly.2016.01.016 |
| 10.1016/j.ssc.2009.04.006 |

| DOI (continued) |
| --- |
| 10.1021/CM500610V |
| 10.1021/acs.chemmater.0c01151 |
| 10.1021/acs.chemmater.5b01464 |
| 10.1021/acs.chemmater.5b02702 |
| 10.1021/acs.chemmater.5b04929 |
| 10.1021/acs.chemmater.6b02109 |
| 10.1021/acs.chemmater.6b05196 |
| 10.1021/acs.chemmater.7b00871 |
| 10.1021/acs.chemmater.7b02724 |
| 10.1021/acs.chemmater.8b01652 |
| 10.1021/acs.chemmater.9b02505 |
| 10.1021/acs.chemmater.9b02990 |
| 10.1021/acs.chemmater.9b04739 |
| 10.1021/acs.inorgchem.5b02647 |
| 10.1021/acs.inorgchem.8b03017 |
| 10.1021/acs.inorgchem.9b00676 |
| 10.1021/acs.inorgchem.9b03142 |
| 10.1021/acs.jpcc.5b06921 |
| 10.1021/acs.jpclett.0c01471 |
| 10.1021/acsami.1c23286 |
| 10.1021/acsami.7b08671 |
| 10.1021/acsomega.8b01952 |
| 10.1021/acsphotonics.8b00844 |
| 10.1021/am2006965 |
| 10.1021/cm051894v |
| 10.1021/cm060898c |
| 10.1021/cm061010n |
| 10.1021/cm203323u |
| 10.1021/cm3000238 |
| 10.1021/cm500116u |
| 10.1021/cm501162n |
| 10.1021/cm502280p |
| 10.1021/cm504604d |
| 10.1021/cm701875e |
| 10.1021/cm801732d |

| DOI (continued) |
| --- |
| 10.1021/cm802394w |
| 10.1021/cm8024796 |
| 10.1021/cm803233d |
| 10.1021/cm9006876 |
| 10.1021/cm9700817 |
| 10.1021/ic00084a038 |
| 10.1021/ic050299s |
| 10.1021/ic102504x |
| 10.1021/ic202340q |
| 10.1021/ic3006053 |
| 10.1021/ic3015578 |
| 10.1021/ic402318k |
| 10.1021/ic500153u |
| 10.1021/ic500963q |
| 10.1021/jacs.7b04338 |
| 10.1021/jacs.8b06021 |
| 10.1021/jp302252k |
| 10.1021/jp309572p |
| 10.1021/jp4062225 |
| 10.1021/jp501949m |
| 10.1021/jp507695n |
| 10.1021/jp508409r |
| 10.1038/NMAT4012 |
| 10.1038/nmat4843 |
| 10.1038/s41467-018-06625-z |
| 10.1038/s41467-019-13293-0 |
| 10.1038/srep03778 |
| 10.1038/srep33283 |
| 10.1039/C0JM04404k |
| 10.1039/C1JM10765H |
| 10.1039/C1JM11018G |
| 10.1039/C1JM12819A |
| 10.1039/C2DT32117C |
| 10.1039/C2JM16882k |
| 10.1039/C2RA00808D |

| DOI (continued) |
|---|
| 10.1039/C2TC00162D |
| 10.1039/C3CE40324F |
| 10.1039/C3DT52832D |
| 10.1039/C3RA47223J |
| 10.1039/C4RA14425B |
| 10.1039/C5CE00020C |
| 10.1039/C5CE01766A |
| 10.1039/C5NJ00297D |
| 10.1039/C5RA20756H |
| 10.1039/C5TC00546A |
| 10.1039/C5TC01151E |
| 10.1039/C6RA14048C |
| 10.1039/C6TC00966B |
| 10.1039/C6TC03818B |
| 10.1039/C7RA08760H |
| 10.1039/C8TC02907E |
| 10.1039/C9TC03919H |
| 10.1039/C9TC05354A |
| 10.1039/b920610h |
| 10.1039/c2tc00731b |
| 10.1039/c3dt51094h |
| 10.1039/c3ra42554a |
| 10.1039/c3tc31798f |
| 10.1039/c4ce00523f |
| 10.1039/c4dt03095h |
| 10.1039/c5cp01860a |
| 10.1039/c5tc01123j |
| 10.1039/c6dt01230b |
| 10.1039/c6ra11681g |
| 10.1039/c6tc00089d |
| 10.1039/c8qi00111a |
| 10.1039/c9dt01252d |
| 10.1039/d2qi01552h |
| 10.1063/1.1544055 |
| 10.1063/1.1935027 |

| DOI (continued) |
|---|
| 10.1063/1.2731685 |
| 10.1063/1.2767182 |
| 10.1063/1.3193549 |
| 10.1088/0022-3727/35/4/312 |
| 10.1088/0022-3727/41/19/195414 |
| 10.1088/1468-6996/14/5/054201 |
| 10.1111/ijac.12474 |
| 10.1111/j.1551-2916.2010.04130.x |
| 10.1111/j.1551-2916.2011.04481.x |
| 10.1111/j.1744-7402.2009.02393.x |
| 10.1111/jace.12032 |
| 10.1111/jace.16537 |
| 10.1149/1.2164693 |
| 10.1149/1.2203101 |
| 10.1149/1.2411413 |
| 10.1149/1.2411498 |
| 10.1149/1.2801380 |
| 10.1149/1.3328530 |
| 10.1149/1.3424899 |
| 10.1149/1.3429887 |
| 10.1149/1.3586043 |
| 10.1149/1.3595434 |
| 10.1149/2.014307jss |
| 10.1149/2.016203jss |
| 10.1149/2.017201esl |
| 10.1149/2.019309jss |
| 10.1149/2.035309jss |
| 10.1364/OE.18.005089 |
| 10.1364/OME.3.000229 |
| 10.1364/ome.4.000280 |
| 10.1524/zkri.220.2.277.59126 |
| 10.1557/jmr.2007.0231 |
| 10.2109/jcersj.113.462 |
| 10.3390/ma6083663 |
| 10.7567/APEX.6.072101 |

Supplementary Table 2: Chemical formulas, ICSD collection codes, and emission wavelengths of phosphors in dataset

| Formula | $\lambda_{em}$ / nm | ICSD Code |
|---|---|---|
| $BaSrMgP_2O_8$:$Eu^{2+}$ | 460.0 | |
| $Sr_3MgSi_2O_8$:$Eu^{2+}$ | 461.6 | 173780 |
| $Ca_9GdP_7O_{28}$:$Eu^{2+}$ | 494.0 | |
| $CaAl_2Si_2O_8$:$Eu^{2+}$ | 430.5 | 252656 |
| $Sr_3B_2O_6$:$Eu^{2+}$ | 582.0 | 93395 |
| $SrLiAl_3N_4$:$Eu^{2+}$ | 650.7 | 427067 |
| SiAlON:$Eu^{2+}$ | 534.5 | |
| $Ba_3Si_6O_{12}N_2$:$Eu^{2+}$ | 526.5 | 259429 |
| $CaSi_2O_2N_2$:$Eu^{2+}$ | 558.7 | 413882 |
| $SrSi_2O_2N_2$:$Eu^{2+}$ | 537.2 | |
| $Ca_8MgSi_4O_{16}C_{12}$:$Eu^{2+}$ | 505.0 | |
| $CaAlSiN_3$:$Eu^{2+}$ | 650.0 | |
| $Ca_2Si_5N_8$:$Eu^{2+}$ | 614.7 | 432574 |
| $Sr_2Si_5N_8$:$Eu^{2+}$ | 621.8 | 401500 |
| $Ba_2Si_5N_8$:$Eu^{2+}$ | 586.5 | 401501 |
| $CaSiN_2$:$Eu^{2+}$ | 623.6 | 170267 |
| $SrSiN_2$:$Eu^{2+}$ | 670.0 | 170266 |
| $BaSiN_2$:$Eu^{2+}$ | 600.0 | 170265 |
| $LiSi_2N_3$:$Eu^{2+}$ | 588.0 | 89524 |
| $SrYSi_4N_7$:$Eu^{2+}$ | 548.0 | 98275 |
| $BaYSi_4N_7$:$Eu^{2+}$ | 503.0 | 98276 |
| $SrSi_6N_8$:$Eu^{2+}$ | 450.0 | 391265 |
| $Al_9O_3N_7$:$Eu^{2+}$ | 482.0 | |
| $SrLi_2Al_2O_2N_2$:$Eu^{2+}$ | 614.0 | |
| $SrLi_2Be_4O_6$:$Eu^{2+}$ | 456.0 | 256229 |
| $Na_3Sc_2P_3O_{12}$:$Eu^{2+}$ | 453.0 | 65406 |
| $NaBaB_9O_{15}$:$Eu^{2+}$ | 416.5 | 93014 |
| $NaK_2Li_{13}Si_4O_{16}$:$Eu^{2+}$ | 528.0 | |
| $BaSr_2SiO_5$:$Eu^{2+}$ | 600.0 | |
| $Rb_2HfSi_2O_7$:$Eu^{2+}$ | 518.0 | |

| Formula | $\lambda_{em}$ / nm | ICSD Code (continued) |
|---|---|---|
| $Cs_2SrP_2O_7$:$Eu^{2+}$ | 543.0 | 39507 |
| $K_3LaSi_2O_7$:$Eu^{2+}$ | 530.0 | |
| $K_3YSi_2O_7$:$Eu^{2+}$ | 619.3 | 430537 |
| $K_3GdSi_2O_7$:$Eu^{2+}$ | 630.0 | 412521 |
| $K_3ScSi_2O_7$:$Eu^{2+}$ | 740.0 | 413432 |
| $Rb_3YSi_2O_7$:$Eu^{2+}$ | 622.0 | |
| $Rb_3GdSi_2O_7$:$Eu^{2+}$ | 550.0 | |
| $Rb_3LuSi_2O_7$:$Eu^{2+}$ | 619.0 | |
| AlN:$Eu^{2+}$ | 480.8 | 608626 |
| $Mg_3N_2$:$Eu^{2+}$ | 589.0 | 679063 |
| $Ba_3Ga_3N_5$:$Eu^{2+}$ | 638.0 | 183911 |
| $Mg_3GaN_3$:$Eu^{2+}$ | 578.0 | |
| $SrAlSiN_3$:$Eu^{2+}$ | 610.0 | |
| $SrAlSi_4N_7$:$Eu^{2+}$ | 633.0 | 163667 |
| $Ba_2AlSi_5N_9$:$Eu^{2+}$ | 584.0 | |
| $Ba_5Al_7Si_{11}N_{25}$:$Eu^{2+}$ | 568.0 | |
| $BaAl_3Si_4N_9$:$Eu^{2+}$ | 500.0 | |
| $SrMg_3SiN_4$:$Eu^{2+}$ | 615.0 | 427076 |
| $BaMg_3SiN_4$:$Eu^{2+}$ | 675.0 | |
| $Li_2Ca_2Mg_2Si_2N_6$:$Eu^{2+}$ | 638.0 | 427078 |
| $CaMg_2Al_2N_4$:$Eu^{2+}$ | 592.0 | |
| $SrMg_2Al_2N_4$:$Eu^{2+}$ | 612.0 | |
| $BaMg_2Ga_2N_4$:$Eu^{2+}$ | 649.0 | |
| $CaLiAl_3N_4$:$Eu^{2+}$ | 668.0 | 194605 |
| $Ca_3MgLi_2Si_2N_6$:$Eu^{2+}$ | 734.0 | 243736 |
| $BaLi_2Al_2Si_2N_6$:$Eu^{2+}$ | 532.0 | |
| $Ba_2LiAlSi_7N_{12}$:$Eu^{2+}$ | 515.0 | |
| $Mg_6AlB_2N_8$:$Eu^{2+}$ | 570.0 | |
| $Mg_7SiB_2N_8$:$Eu^{2+}$ | 560.0 | |
| $Mg_3BN_3$:$Eu^{2+}$ | 704.3 | 79623 |
| $Mg_3GaBN_4$:$Eu^{2+}$ | 600.0 | |
| $BaSi_2O_2N_2$:$Eu^{2+}$ | 493.8 | 173758 |
| $La_4Si_{12}O_3N_{18}$:$Eu^{2+}$ | 565.0 | |
| $Ce_4Si_{12}O_3N_{18}$:$Eu^{2+}$ | 581.0 | |
| $Ca_{15}Si_{20}O_{10}N_{30}$:$Eu^{2+}$ | 641.0 | |

| Formula | $\lambda_{em}$ / nm | ICSD Code (continued) |
|---|---|---|
| $Sr_3Si_2O_4N_2:Eu^{2+}$ | 600.0 | |
| $BaSi_6N_8O:Eu^{2+}$ | 500.0 | 415272 |
| $Si_6N_8:Eu^{2+}$ | 535.0 | 74742 |
| $Sr_{14}Si_{68}Al_6N_{106}:Eu^{2+}$ | 508.0 | |
| $Sr_5Al_5Si_{21}N_{35}O_2:Eu^{2+}$ | 510.0 | |
| $Sr_3Si_{13}Al_3O_2N_{21}:Eu^{2+}$ | 515.0 | |
| $SrSiAl_2O_3N_2:Eu^{2+}$ | 472.0 | 408170 |
| $SrSi_9Al_{19}ON_{31}:Eu^{2+}$ | 450.0 | |
| $Sr_3Si_8O_7N_8:Eu^{2+}$ | 465.0 | |
| $Sr_2Si_7Al_3ON_{13}:Eu^{2+}$ | 615.0 | |
| $SrCN_2:Eu^{2+}$ | 603.0 | 59860 |
| $Sr_2B_2Si_2Al_2N_8:Eu^{2+}$ | 598.0 | |
| $CaP_2N_4:Eu^{2+}$ | 575.0 | 425997 |
| $SrP_2N_4:Eu^{2+}$ | 529.0 | 249348 |
| $BaP_2N_4:Eu^{2+}$ | 460.0 | 414350 |
| $BaSr_2P_6N_{12}:Eu^{2+}$ | 450.0 | 415716 |
| $Ca_2PO_3N:Eu^{2+}$ | 526.5 | 430215 |
| $Ba_3P_5N_{10}Cl:Eu^{2+}$ | 439.0 | |
| $Ba_3P_5N_{10}Br:Eu^{2+}$ | 472.0 | |
| $Ba_3P_5N_{10}I:Eu^{2+}$ | 494.0 | |
| $CaAl_2O_4:Eu^{2+}$ | 438.5 | 172780 |
| $BaAl_2O_4:Eu^{2+}$ | 515.0 | 21080 |
| $Sr_4Al_{14}O_{25}:Eu^{2+}$ | 489.5 | 27744 |
| $SrAl_4O_7:Eu^{2+}$ | 480.0 | 16751 |
| $SrAl_{12}O_{19}:Eu^{2+}$ | 397.5 | 2006 |
| $Ca_{12}Al_{14}O_{33}:Eu^{2+}$ | 440.0 | |
| $Sr_3Al_2O_6:Eu^{2+}$ | 510.0 | 71860 |
| $SrMgAl_{10}O_{17}:Eu^{2+}$ | 462.5 | |
| $BaMgAl_{10}O_{17}:Eu^{2+}$ | 452.5 | |
| $Sr_2MgSi_2O_7:Eu^{2+}$ | 485.2 | 261226 |
| $Ba_2MgSi_2O_7:Eu^{2+}$ | 501.2 | 81117 |
| $Ca_3MgSi_2O_8:Eu^{2+}$ | 472.0 | 43078 |
| $Ba_3MgSi_2O_8:Eu^{2+}$ | 439.0 | 195483 |
| $CaMgSi_2O_6:Eu^{2+}$ | 445.0 | 31116 |
| $Sr_3Al_{10}SiO_{20}:Eu^{2+}$ | 465.0 | |

| Formula | $\lambda_{em}$ / nm | ICSD Code (continued) |
|---|---|---|
| $Sr_2Al_2SiO_7:Eu^{2+}$ | 503.8 | |
| $Sr_2ZnSi_2O_7:Eu^{2+}$ | 465.0 | 247476 |
| $CaS:Eu^{2+}$ | 654.0 | 682350 |
| $CaGa_2S_4:Eu^{2+}$ | 556.5 | 619292 |
| $Sr_2P_2O_7:Eu^{2+}$ | 420.0 | 34467 |
| $Ca_2P_2O_7:Eu^{2+}$ | 419.0 | 22225 |
| $SrMg_2P_2O_8:Eu^{2+}$ | 405.0 | |
| $CaAl_2B_2O_7:Eu^{2+}$ | 465.0 | 86785 |
| $SrB_2O_4:Eu^{2+}$ | 442.0 | 203226 |
| $KF:Eu^{2+}$ | 427.0 | 61558 |
| $NaF:Eu^{2+}$ | 422.0 | 674962 |
| $BaAlF_5:Eu^{2+}$ | 360.0 | 80563 |
| $BaCaAlF_7:Eu^{2+}$ | 356.0 | 281208 |
| $BaBeF_4:Eu^{2+}$ | 378.0 | 414412 |
| $Ba_2Mg_3F_{10}:Eu^{2+}$ | 382.0 | 50228 |
| $BaMgF_4:Eu^{2+}$ | 415.0 | 182599 |
| $BaF_2:Eu^{2+}$ | 403.0 | 41649 |
| $LiBaAlF_6:Eu^{2+}$ | 361.0 | 260011 |
| $SrAlF_5:Eu^{2+}$ | 362.0 | 411509 |
| $Sr_2AlF_7:Eu^{2+}$ | 390.0 | |
| $SrCaAlF_7:Eu^{2+}$ | 380.0 | |
| $SrBeF_4:Eu^{2+}$ | 373.0 | 404396 |
| $SrMgF_4:Eu^{2+}$ | 427.0 | 86248 |
| $EuMgF_4:Eu^{2+}$ | 437.0 | 86246 |
| $SrF_2:Eu^{2+}$ | 416.0 | 168801 |
| $CsSrF_3:Eu^{2+}$ | 426.0 | 49578 |
| $RbSrF_3:Eu^{2+}$ | 424.0 | 680499 |
| $CaAlF_5:Eu^{2+}$ | 386.0 | 69563 |
| $Ca_2AlF_7:Eu^{2+}$ | 400.0 | 121553 |
| $CaBeF_4:Eu^{2+}$ | 390.0 | |
| $CaMgF_4:Eu^{2+}$ | 430.0 | |
| $CaF_2:Eu^{2+}$ | 424.0 | 51237 |
| $RbCaF_3:Eu^{2+}$ | 461.0 | 201253 |
| $KCaF_3:Eu^{2+}$ | 431.0 | 679549 |
| $LiCaAlF_6:Eu^{2+}$ | 371.0 | 39699 |

| Formula | $\lambda_{em}$ / nm | ICSD Code (continued) |
|---|---|---|
| $MgF_2:Eu^{2+}$ | 438.0 | 9164 |
| $CsMgF_3:Eu^{2+}$ | 360.0 | 290359 |
| $RbMgF_3:Eu^{2+}$ | 365.0 | 49585 |
| $KMgF_3:Eu^{2+}$ | 342.0 | 40476 |
| $NaMgF_3:Eu^{2+}$ | 365.0 | 193089 |
| $BaCaLu_2F_{10}:Eu^{2+}$ | 401.0 | |
| $Ba_{12}F_{19}Cl_5:Eu^{2+}$ | 440.0 | 183927 |
| $BaFCl:Eu^{2+}$ | 387.0 | 201518 |
| $SrFCl:Eu^{2+}$ | 388.0 | 159278 |
| $EuFCl:Eu^{2+}$ | 417.0 | 108938 |
| $CaFCl:Eu^{2+}$ | 396.0 | 1130 |
| $CsCl:Eu^{2+}$ | 441.0 | 673994 |
| $RbCl:Eu^{2+}$ | 417.0 | 61521 |
| $KCl:Eu^{2+}$ | 423.0 | 290513 |
| $NaCl:Eu^{2+}$ | 427.0 | 674961 |
| $LiCl:Eu^{2+}$ | 424.0 | 671518 |
| $BaCl_2:Eu^{2+}$ | 398.0 | 2190 |
| $BaZnCl_4:Eu^{2+}$ | 399.0 | 410194 |
| $SrCl_2:Eu^{2+}$ | 410.0 | 31172 |
| $EuCl_2:Eu^{2+}$ | 413.0 | 60318 |
| $SrZnCl_4:Eu^{2+}$ | 404.0 | 410191 |
| $CaCl_2:Eu^{2+}$ | 429.0 | 246417 |
| $LaCl_3:Eu^{2+}$ | 409.0 | 23146 |
| $BaFBr:Eu^{2+}$ | 391.0 | 155005 |
| $EuFBr:Eu^{2+}$ | 393.0 | 432469 |
| $CsBr:Eu^{2+}$ | 441.0 | 682442 |
| $RbBr:Eu^{2+}$ | 416.0 | 61522 |
| $KBr:Eu^{2+}$ | 425.0 | 290550 |
| $NaBr:Eu^{2+}$ | 429.0 | 674960 |
| $BaBr_2:Eu^{2+}$ | 407.0 | 262675 |
| $SrBr_2:Eu^{2+}$ | 411.0 | 15972 |
| $EuBr_2:Eu^{2+}$ | 421.0 | 60316 |
| $CaBr_2:Eu^{2+}$ | 433.0 | 173969 |
| $CsCdBr_3:Eu^{2+}$ | 476.0 | 681818 |
| $Rb_2ZnBr_4:Eu^{2+}$ | 435.0 | 97854 |

| Formula | $\lambda_{em}$ / nm | ICSD Code (continued) |
|---|---|---|
| $CsI:Eu^{2+}$ | 447.0 | 677210 |
| $RbI:Eu^{2+}$ | 426.0 | 61523 |
| $KI:Eu^{2+}$ | 432.0 | 61555 |
| $NaI:Eu^{2+}$ | 439.0 | 674963 |
| $SrI_2:Eu^{2+}$ | 431.0 | 203137 |
| $EuI_2:Eu^{2+}$ | 435.0 | 260561 |
| $CsEu_2I_5$ | 440.0 | 41099 |
| $CsEuI_3:Eu^{2+}$ | 449.0 | |
| $RbEu_2I_5$ | 443.0 | 41098 |
| $RbEuI_3:Eu^{2+}$ | 459.0 | |
| $KEu_2I_5$ | 447.0 | 41100 |
| $CaI_2:Eu^{2+}$ | 467.0 | 682421 |
| $Ba_5(PO_4)_3F:Eu^{2+}$ | 432.0 | |
| $Sr_5(PO_4)_3F:Eu^{2+}$ | 438.0 | 163792 |
| $Ca_5(PO_4)_3F:Eu^{2+}$ | 448.0 | 236762 |
| $Ba_5(PO_4)_3Cl:Eu^{2+}$ | 415.5 | 241980 |
| $Ca_2PO_4Cl:Eu^{2+}$ | 449.5 | 15316 |
| $Ba_2B_5O_9Cl:Eu^{2+}$ | 409.5 | 409640 |
| $Sr_2B_5O_9Cl:Eu^{2+}$ | 423.5 | 246037 |
| $Eu_2B_5O_9Cl$ | 430.0 | 86477 |
| $Ca_2B_5O_9Cl:Eu^{2+}$ | 440.0 | |
| $Ca_5(BO_3)_2Cl:Eu^{2+}$ | 587.0 | |
| $Ba_2Y(BO_3)_2Cl:Eu^{2+}$ | 538.0 | 262072 |
| $Sr_4Si_3O_8Cl_4:Eu^{2+}$ | 500.0 | |
| $Sr_2SiO_3Cl_2:Eu^{2+}$ | 490.0 | 51594 |
| $Eu_2SiO_3Cl_2$ | 505.0 | 400126 |
| $Ba_5SiO_4Cl_6:Eu^{2+}$ | 440.3 | 67566 |
| $Eu_5SiO_4Cl_6:Eu^{2+}$ | 450.0 | 400127 |
| $Ca_3SiO_4Cl_2:Eu^{2+}$ | 505.0 | 9088 |
| $Ba_4OCl_6:Eu^{2+}$ | 452.0 | 408175 |
| $Sr_5(PO_4)_3Br:Eu^{2+}$ | 452.0 | 184830 |
| $Ba_2B_5O_9Br:Eu^{2+}$ | 422.5 | |
| $Sr_2B_5O_9Br:Eu^{2+}$ | 427.5 | |
| $Eu_2B_5O_9Br$ | 435.0 | 16364 |
| $Ca_2B_5O_9Br:Eu^{2+}$ | 441.5 | 166560 |

| Formula | $\lambda_{em}$ / nm | ICSD Code (continued) |
| --- | --- | --- |
| $Ba_5SiO_4Br_6$:$Eu^{2+}$ | 441.0 | 73365 |
| $Ba_4OBr_6$:$Eu^{2+}$ | 454.0 | 391435 |
| $Sr_4OBr_6$:$Eu^{2+}$ | 450.0 | 418452 |
| $Rb_2SO_4$:$Eu^{2+}$ | 396.0 | 71527 |
| $K_2SO_4$:$Eu^{2+}$ | 405.0 | 27956 |
| $LiNaSO_4$:$Eu^{2+}$ | 419.0 | 67703 |
| $BaSO_4$:$Eu^{2+}$ | 374.0 | 33731 |
| $BaMg(SO_4)_2$:$Eu^{2+}$ | 361.0 | |
| $SrSO_4$:$Eu^{2+}$ | 376.0 | 85809 |
| $CaSO_4$:$Eu^{2+}$ | 386.0 | 24473 |
| $K_2Ca_2(SO_4)_3$:$Eu^{2+}$ | 413.0 | 243319 |
| $MgSO_4$:$Eu^{2+}$ | 378.0 | 27130 |
| $CaCO_3$:$Eu^{2+}$ | 450.0 | 133254 |
| $Ba(PO_3)_2$:$Eu^{2+}$ | 375.0 | 15714 |
| $Ba_2MgP_4O_{13}$:$Eu^{2+}$ | 403.0 | |
| $BaMgP_2O_7$:$Eu^{2+}$ | 402.0 | 39398 |
| $BaCaP_2O_7$:$Eu^{2+}$ | 435.0 | 184750 |
| $BaSrP_2O_7$:$Eu^{2+}$ | 435.0 | |
| $Ba_2P_2O_7$:$Eu^{2+}$ | 406.0 | 261125 |
| $Sr_3P_4O_{13}$:$Eu^{2+}$ | 415.0 | 99588 |
| $Sr_2Mg_3P_4O_{15}$:$Eu^{2+}$ | 440.0 | |
| $SrMgP_2O_7$:$Eu^{2+}$ | 394.0 | 280782 |
| $Mg_2P_2O_7$:$Eu^{2+}$ | 424.0 | 20295 |
| $BaMg_2(PO_4)_2$:$Eu^{2+}$ | 418.0 | |
| $Ba_2Ca(PO_4)_2$:$Eu^{2+}$ | 463.0 | |
| $Ba_3(PO_4)_2$:$Eu^{2+}$ | 415.0 | 30634 |
| $KBaPO_4$:$Eu^{2+}$ | 420.0 | 23884 |
| $NaBaPO_4$:$Eu^{2+}$ | 442.5 | |
| $LiBaPO_4$:$Eu^{2+}$ | 483.0 | 36801 |
| $Sr_3(PO_4)_2$:$Eu^{2+}$ | 411.0 | 18109 |
| $KSrPO_4$:$Eu^{2+}$ | 429.0 | 83598 |
| $NaSrPO_4$:$Eu^{2+}$ | 463.8 | |
| $LiSrPO_4$:$Eu^{2+}$ | 459.7 | 258641 |
| $Ca_3(PO_4)_2$:$Eu^{2+}$ | 433.7 | 200202 |
| $Ca_3Mg_3(PO_4)_4$:$Eu^{2+}$ | 434.0 | 23642 |

| Formula | $\lambda_{em}$ / nm | ICSD Code (continued) |
|---|---|---|
| $KCaPO_4:Eu^{2+}$ | 503.8 | |
| $NaCaPO_4:Eu^{2+}$ | 505.5 | 35629 |
| $LiCaPO_4:Eu^{2+}$ | 475.0 | 66387 |
| $Mg_3(PO_4)_2:Eu^{2+}$ | 425.0 | 31005 |
| $Sr_5(PO_4)_3OH:Eu^{2+}$ | 447.0 | |
| $BaB_8O_{13}:Eu^{2+}$ | 390.0 | 26203 |
| $BaLiB_9O_{15}:Eu^{2+}$ | 383.0 | 95115 |
| $SrB_4O_7:Eu^{2+}$ | 367.0 | 185674 |
| $EuB_4O_7:Eu^{2+}$ | 370.0 | 30507 |
| $SrLiB_9O_{15}:Eu^{2+}$ | 385.0 | 93015 |
| $Ca_2B_5SiO_9(OH)_5:Eu^{2+}$ | 455.0 | 202665 |
| $Ba_2Ca(B_3O_6)_2:Eu^{2+}$ | 450.0 | 30890 |
| $Ba_2Mg(B_3O_6)_2:Eu^{2+}$ | 425.0 | 290356 |
| $CaB_2O_4:Eu^{2+}$ | 368.0 | 40889 |
| $BaBe_2(BO_3)_2:Eu^{2+}$ | 392.5 | 254360 |
| $Sr_3Al_6(BO_3)_8:Eu^{2+}$ | 420.0 | |
| $BaBPO_5:Eu^{2+}$ | 381.0 | 95116 |
| $BaAl_3BO_7:Eu^{2+}$ | 360.0 | |
| $SrAl_3BO_7:Eu^{2+}$ | 400.0 | |
| $SrBPO_5:Eu^{2+}$ | 388.0 | 87894 |
| $SrAl_2B_2O_7:Eu^{2+}$ | 409.0 | 89423 |
| $Sr_2Al_2B_2O_8:Eu^{2+}$ | 415.0 | 28107 |
| $CaAl_3BO_7:Eu^{2+}$ | 420.0 | |
| $CaBPO_5:Eu^{2+}$ | 403.0 | 87893 |
| $BaZrSi_3O_9:Eu^{2+}$ | 475.0 | |
| $SrSiO_3:Eu^{2+}$ | 440.0 | 248973 |
| $CaSiO_3:Eu^{2+}$ | 465.0 | 240413 |
| $BaBe_2Si_2O_7:Eu^{2+}$ | 374.0 | 151563 |
| $BaMg_2Si_2O_7:Eu^{2+}$ | 400.0 | 420258 |
| $SrBe_2Si_2O_7:Eu^{2+}$ | 360.0 | |
| $BaAl_2(SiO_4)_2:Eu^{2+}$ | 427.0 | 191252 |
| $BaMg(SiO_4):Eu^{2+}$ | 437.0 | 73776 |
| $EuAl_2(SiO_4)_2:Eu^{2+}$ | 520.0 | |
| $Eu_2(SiO_4)$ | 564.0 | 1510 |
| $Li_4Sr_2Ca(SiO_4)_2:Eu^{2+}$ | 428.0 | |

| Formula | $\lambda_{em}$ / nm | ICSD Code (continued) |
|---|---|---|
| $CaB(OH)(SiO_4)$:$Eu^{2+}$ | 446.0 | 168616 |
| $CaB_2O(Si_2O_7)$:$Eu^{2+}$ | 431.0 | 244766 |
| $Sr_3SiO_5$:$Eu^{2+}$ | 561.7 | 18151 |
| $Ca_3SiO_5$:$Eu^{2+}$ | 510.0 | 81100 |
| $Al_2O_3$:$Eu^{2+}$ | 460.0 | 33639 |
| $RbAl_{11}O_{17}$:$Eu^{2+}$ | 442.0 | |
| $KAl_{11}O_{17}$:$Eu^{2+}$ | 445.0 | |
| $NaAl_{11}O_{17}$:$Eu^{2+}$ | 464.0 | 16933 |
| $BaAlGaO_4$:$Eu^{2+}$ | 532.5 | |
| $BaAl_{12}O_{19}$:$Eu^{2+}$ | 440.0 | |
| $BaMg_2Al_{14}O_{24}$:$Eu^{2+}$ | 447.0 | |
| $BaMg_2Al_{16}O_{27}$:$Eu^{2+}$ | 449.0 | |
| $SrCaAl(AlSiO_7)$:$Eu^{2+}$ | 532.0 | |
| $Sr_2Al_6O_{11}$:$Eu^{2+}$ | 460.0 | 97713 |
| $EuAl_{12}O_{19}$:$Eu^{2+}$ | 420.0 | |
| $EuMgAl_{10}O_{17}$:$Eu^{2+}$ | 475.0 | |
| $SrMg_2Al_{10}O_{18}$:$Eu^{2+}$ | 470.0 | |
| $Ca_2Al(AlSiO_7)$:$Eu^{2+}$ | 440.0 | 24588 |
| $CaAl_{12}O_{19}$:$Eu^{2+}$ | 412.0 | 34394 |
| $MgAl_2O_4$:$Eu^{2+}$ | 485.0 | 157186 |
| $LaMgAl_{11}O_{19}$:$Eu^{2+}$ | 450.0 | |
| $EuAlO_3$:$Eu^{2+}$ | 518.0 | 109353 |
| $BaZrO_3$:$Eu^{2+}$ | 494.0 | 674065 |
| $SrO$:$Eu^{2+}$ | 625.0 | 670284 |
| $CaO$:$Eu^{2+}$ | 738.0 | 682348 |
| $Na_2Si_2S_5$:$Eu^{2+}$ | 487.0 | 166532 |
| $BaSi_2S_5$:$Eu^{2+}$ | 509.0 | |
| $SrSi_2S_5$:$Eu^{2+}$ | 488.0 | |
| $Na_4SiS_4$:$Eu^{2+}$ | 459.0 | 31813 |
| $Sr_2SiS_4$:$Eu^{2+}$ | 543.0 | 650888 |
| $Mg_2SiS_4$:$Eu^{2+}$ | 660.0 | 642791 |
| $BaAl_4S_7$:$Eu^{2+}$ | 470.0 | 33237 |
| $BaAl_2S_4$:$Eu^{2+}$ | 473.0 | 35136 |
| $Ba_2Al_2S_5$:$Eu^{2+}$ | 487.0 | |
| $Ba_4Al_2S_7$:$Eu^{2+}$ | 534.0 | |

| Formula | $\lambda_{em}$ / nm | ICSD Code (continued) |
|---|---|---|
| $Ba_5Al_2S_8$:$Eu^{2+}$ | 540.0 | |
| $BaGa_4S_7$:$Eu^{2+}$ | 482.0 | 162960 |
| $BaGa_2S_4$:$Eu^{2+}$ | 497.0 | 615871 |
| $Ba_3Ga_2S_6$:$Eu^{2+}$ | 538.0 | 201421 |
| $SrAl_2S_4$:$Eu^{2+}$ | 496.0 | 609259 |
| $Sr_2Al_2S_5$:$Eu^{2+}$ | 522.0 | |
| $SrGa_2S_4$:$Eu^{2+}$ | 533.5 | 635274 |
| $Sr_2Ga_2S_5$:$Eu^{2+}$ | 553.0 | 635273 |
| $CaAl_2S_4$:$Eu^{2+}$ | 516.0 | 46016 |
| $ZnGa_2S_4$:$Eu^{2+}$ | 537.0 | 635300 |
| BaS:$Eu^{2+}$ | 572.0 | 683800 |
| SrS:$Eu^{2+}$ | 618.0 | 52111 |
| MgS:$Eu^{2+}$ | 592.0 | 675092 |
| $SrY_2S_4$:$Eu^{2+}$ | 645.0 | 80295 |
| $BaIn_2S_4$:$Eu^{2+}$ | 680.0 | 46020 |
| $SrIn_2S_4$:$Eu^{2+}$ | 640.0 | 300176 |
| $EuGa_2Se_4$:$Eu^{2+}$ | 528.0 | 631269 |
| $CaGa_2Se_4$:$Eu^{2+}$ | 562.0 | 24387 |
| SrSe:$Eu^{2+}$ | 571.0 | 674020 |
| CaSe:$Eu^{2+}$ | 597.0 | 682352 |
| $LaEuSi_2N_3O_2$:$Eu^{2+}$ | 650.0 | |
| $LaSi_3N_5$:$Eu^{2+}$ | 549.0 | 130022 |
| $Li_2SrSiO_4$:$Eu^{2+}$ | 558.0 | 167334 |
| $Ca_{12}Al_{14}O_{32}F_2$:$Eu^{2+}$ | 440.0 | |
| $Sr_3Y_2(Si_3O_9)_2$:$Eu^{2+}$ | 474.0 | |
| $Ca_1Sr_0LaGa_3S_6O$: 0.05 $Eu^{2+}$ | 547.5 | |
| $Sr_8MgY(PO_4)_7$:$Eu^{2+}$ | 518.0 | |
| $Sr_3Ce(PO_4)_3$:$Eu^{2+}$ | 535.0 | |
| $Ca_4(PO_4)_2O$:$Eu^{2+}$ | 661.7 | 160461 |
| $Sr_4(PO_4)_2O$:$Eu^{2+}$ | 687.5 | |
| $Sr_3Al_2O_5Cl_2$:$Eu^{2+}$ | 614.0 | 68365 |
| AlON:$Eu^{2+}$ | 429.3 | |
| $Ca_9Mg(PO_4)_6F_2$:$Eu^{2+}$ | 405.0 | |
| $Ca_4Si_2O_7F_2$:$Eu^{2+}$ | 400.0 | 64710 |
| $KCaY(PO_4)_2$:$Eu^{2+}$ | 480.0 | |

| Formula | $\lambda_{em}$ / nm | ICSD Code (continued) |
|---|---|---|
| $BaMg_2Al_6Si_9O_{30}$:$Eu^{2+}$ | 376.0 | |
| $KCaGd(PO_4)_2$:$Eu^{2+}$ | 463.0 | |
| $RbLi(Li_3SiO_4)_2$:$Eu^{2+}$ | 530.0 | 33864 |
| $BaSrSiO_4$:$Eu^{2+}$ | 512.0 | |
| $Cs_2Ba_1Ca_0P_2O_7$: 0.01 $Eu^{2+}$ | 530.0 | 252184 |
| $Cs_2Ba_0Ca_1P_2O_7$: 0.01 $Eu^{2+}$ | 574.5 | |
| $Cs_2Sr_1Ca_0P_2O_7$: 0.01 $Eu^{2+}$ | 543.0 | 39507 |
| $Cs_2Sr_0Ca_1P_2O_7$: 0.01 $Eu^{2+}$ | 571.0 | |
| $Cs_2Ba_{0.2}Sr_{0.8}P_2O_7$: 0.01 $Eu^{2+}$ | 538.0 | 39507 |
| $Sr_{0.25}Ba_{0.75}Si_2O_2N_2$:$Eu^{2+}$ | 472.0 | 173758 |
| $Ba_3La_6(SiO_4)_6$:$Eu^{2+}$ | 507.0 | |
| $Ca_3Si_2O_7$:$Eu^{2+}$ | 610.0 | 2282 |
| BSP:$Eu^{2+}$, $Tb_3{}^+$ | 518.0 | |
| $NaCaBO_3$:$Eu^{2+}$ | 477.0 | |
| $Sr_{18}Mg_3(PO_4)_{14}$:$_1$%$Eu^{2+}$ | 420.0 | |
| $Na_2BaCa_1Sr_0(PO_4)_2$: 0.03 $Eu^{2+}$ | 448.0 | |
| $Na_2BaCa(PO_4)_2$: 0.03 $Eu^{2+}$ | 448.0 | |
| $Na_2BaCa_{0.2}Sr_{0.8}(PO_4)_2$: 0.03 $Eu^{2+}$ | 428.0 | |
| $Ca_2ZnSi_2O_7$:$Eu^{2+}$ | 600.0 | 18114 |
| $Sr_5(PO_4)_3Cl_0$:$Eu^{2+}$ | 447.0 | |
| $Ba_5(PO_4)_3Cl_0$:$Eu^{2+}$ | 436.0 | |
| $Ca_2BO_3Cl$: 0.015 $Eu^{2+}$ | 575.0 | 16032 |
| $CaZrSi_2O_7$:$Eu^{2+}$ | 512.0 | 203131 |
| $CaLaGa_3S_7$:$Eu^{2+}$ | 554.0 | |
| $Sr_6BP_5O_{20}$:$Eu^{2+}$ | 480.0 | 172402 |
| $SrLu_2O_4$:$Eu^{2+}$ | 610.0 | 14740 |
| $Sr_3YNa(PO_4)_3F$:$Eu^{2+}$ | 456.0 | 4683 |
| SYNPF: 0.1 $Eu^{2+}$ | 456.0 | |
| $Ba_{0.94}Zn_2(BO_3)_2$: 0.06 $Eu^{2+}$ | 490.0 | 72193 |
| $Ba_9Sc_2Si_6O_{24}$:$Eu^{2+}$ | 486.0 | 252602 |
| BSSO:$Eu_2$ | 512.0 | |
| $Cs_2CaP_2O_7$:$Eu^{2+}$, $Tb_3{}^+$ | 590.0 | |
| $NaAlSiO_4$: 0.1 $Eu^{2+}$ | 551.0 | 12645 |
| $KBa_1ScSi_3O_9$:$Eu_2$ | 521.0 | |
| $BaZn_2Si_2O_7$:$Eu^{2+}$ | 522.0 | 88589 |

| Formula | $\lambda_{em}$ / nm | ICSD Code (continued) |
|---|---|---|
| $Ca_1Eu_0SiN_2$:$Eu^{2+}$ | 628.0 | 170267 |
| $YAl_3(BO_3)_4$:$Eu^{2+}$ | 425.0 | 91962 |
| $CaAlSi_1N_3O_0$:$Eu^{2+}$ | 640.0 | |
| $CaLaGa_3S_6O$: 0.05 $Eu^{2+}$ | 560.0 | |
| $SrLaGa_3S_6O$: 0.10 $Eu^{2+}$ | 540.0 | |
| $Ca_{7.9}MgLa(PO_4)_7$: 0.1 $Eu^{2+}$ | 505.0 | |
| $Ca_{7.9}MgLa_0Y_1(PO_4)_7$: 0.1 $Eu^{2+}$ | 484.0 | |
| $Ca_{7.88}MgY(PO_4)_7$: 0.12 $Eu^{2+}$ | 474.4 | |
| $(Ca_{0.99})_9(Y_1La_0)(PO_4)_7$: 0.01 $Eu^{2+}$ | 485.0 | |
| $(Ca_{0.99})_9(Y_0La_1)(PO_4)_7$: 0.01 $Eu^{2+}$ | 502.0 | |
| $Ca_7(PO_4)_2(SiO_4)_2$:$Eu^{2+}$ | 522.0 | |
| $Ba_9Y_2Si_6O_{24}$:$Eu^{2+}$ | 503.0 | 237604 |
| $Ba[(Mg_{0.2}Li_{1.8})(Al_{2.2}Si_{1.8})N_6]$:$Eu^{2+}$ | 561.0 | |
| $CaSi_9Al_3ON_{15}$:$Eu^{2+}$ | 581.0 | |
| Ca(20) Li(8) $[Al_{39}N_{55}]$:$Eu^{2+}$ | 647.0 | |
| $Li_2(Ca_{1.88}Sr_{0.12})[Mg_2Si_2N_6]$:$Eu^{2+}$ | 634.0 | 427078 |
| $Ca_9Lu(PO_4)_7$:$Eu^{2+}$ | 480.0 | |
| $Ca_{10}Li(PO_4)_7$: 0.001 $Eu^{2+}$ | 414.0 | 257128 |
| $Ca_{10}K(PO_4)_7$: 0.001 $Eu^{2+}$ | 440.0 | 245053 |
| $Sr_2AlSi_2O_6N$:$Eu^{2+}$ | 600.0 | |
| $Sr_2Al_2Si_1O_7N_0$:$Eu^{2+}$ | 513.0 | |
| $Sr_2Ca_0AlSi_2O_6N$:$Eu^{2+}$ | 600.0 | |
| $Sr_0Ca_2AlSi_2O_6N$:$Eu^{2+}$ | 525.0 | |
| $Lu_2CaMg_2Si_3O_{12}$:$Eu^{2+}$ | 365.0 | |
| $Y_2Mg_2Al_2Si_2O_{12}$:$Eu^{2+}$ | 436.0 | |
| $Lu_2MgAl_4SiO_{12}$:$_1$%$Eu^{2+}$ | 463.0 | |
| $Lu_2Mg_{0.4}Ca_{0.6}Al_4SiO_{12}$:$_1$%$Eu^{2+}$ | 495.5 | |
| $K_2HfSi_3O_9$:$_1$%$Eu^{2+}$ | 493.0 | 9253 |
| $Ba_2SiO_4$:$Eu^{2+}$ | 516.5 | 6246 |
| $MgSiN_2$:$Eu^{2+}$ | 517.0 | 186509 |
| $Sr_{0.98}Ca_{0.02}Si_2N_2O_2$:$Eu_2$% | 543.0 | |
| $Ba_2Mg(BO_3)_2$:$Eu^{2+}$ | 617.0 | 75986 |
| $Ba_2Ca(BO_3)_2$:$Eu^{2+}$ | 530.0 | 80429 |
| $(Ca_{0.993}Mg_0)_9Y(PO_4)_7$: 0.007 $Eu^{2+}$ | 435.0 | |
| $(Ca_{0.993}Sr_0)_9Y(PO_4)_7$: 0.007 $Eu^{2+}$ | 486.0 | |

| Formula | $\lambda_{em}$ / nm | ICSD Code (continued) |
|---|---|---|
| $RbBaPO_4$:$Eu^{2+}$ | 430.0 | 72001 |
| $CaAlSiNS_3$:$Eu^{2+}$(CASN) | 645.0 | |
| $CaZr(PO_4)_2$:$Eu^{2+}$ | 470.0 | 150877 |
| $BaLa_2Si_2S_8$:$Eu^{2+}$ | 645.0 | |
| $Ba_{1.305}Ca_{0.38}Mg_{0.3}SiO_4$: 0.015 $Eu^{2+}$ | 475.0 | 95755 |
| BCS:$Eu^{2+}$ | 495.0 | |
| $Ga_2S_3$:$Eu^{2+}$ | 586.0 | 635243 |

Supplementary Table 3: Evaluating the performance of GPT-n models with varying context lengths on Ref. [1]

| Chemical formula | Emission peak / nm |
|---|---|
| GPT-4, 1k context length | |
| $M_2SiO_4:Eu^{2+}$ (M = Ba, Ca) | 500 |
| $M_2SiO_4:Eu^{2+}$ (M = Sr) | 575 |
| $M_2SiO_4:Ce^{3+}$ (M = Ba, Sr) | 390 |
| $Ca_2SiO_4:Ce^{3+}$ | Yellow luminescence (specific nm not provided) |
| $Ca_3SiO_5:Eu^{2+}$ | 500-600 |
| $Sr_3SiO_5:Eu^{2+}$ | 500-600 |
| $Ba_3SiO_5:Eu^{2+}$ | 500-600 |
| $Sr_3SiO_5:Ce^{3+}$ | 530-630 |
| $Ca_2MgSi_2O_7:Eu^{2+}$ | 475 |
| $Sr_2MgSi_2O_7:Eu^{2+}$ | 540 |
| $Ba_2MgSi_2O_7:Eu^{2+}$ | 500 |
| $Ba_3MgSi_2O_8:Eu^{2+}$ | 440 |
| $Ca_3MgSi_2O_8:Eu^{2+}$ | 475 |
| YAG:Ce | 540 |
| Ce-doped $Ca_3Sc_2Si_3O_{12}$ | 505 |
| $Ca_2Si_5N_8:Eu^{2+}$ | 605 |
| $Sr_2Si_5N_8:Eu^{2+}$ | 620 |
| $Ba_2Si_5N_8:Eu^{2+}$ | 580 |
| $Ca_2Si_5N_8:Ce^{3+}$ | 470 |
| $Sr_2Si_5N_8:Ce^{3+}$ | 553 |
| $Ba_2Si_5N_8:Ce^{3+}$ | 451 |
| $CaSi_2O_2N_2:Eu^{2+}$ | 560 |
| $SrSi_2O_2N_2:Eu^{2+}$ | 530-570 |
| $BaSi_2O_2N_2:Eu^{2+}$ | 500 |
| $LaSr_2AlO_5:Ce^{3+}$ | 556 |
| $Sr_3(AlO_4F)_{0.5}(SiO_5)_{0.5}:Ce^{3+}$ | 525 |
| $Sr_2Ba(AlO_4F)_{0.5}(SiO_5)_{0.5}:Ce^{3+}$ | 539 |
| GPT-4, 2k context length | |
| $Ca_3SiO_5:Eu^{2+}$ | 500-600 |

| Chemical formula | Emission peak / nm (continued) |
|---|---|
| $Ca_3SiO_5:Ce^{3+}$ | ∼530 |
| $Sr_3SiO_5:Ce^{3+}$ | ∼560 |
| $Ca_2MgSi_2O_7:Eu^{2+}$ | 475 |
| $Sr_2MgSi_2O_7:Eu^{2+}$ | 540 |
| $Ba_2MgSi_2O_7:Eu^{2+}$ | 500 |
| $Ba_3MgSi_2O_8:Eu^{2+}$ | 440 |
| $Ca_3MgSi_2O_8:Eu^{2+}$ | 475 |
| YAG:Ce | 540 |
| $Ca_3Sc_2Si_3O_{12}$:Ce | 505 |
| $Ca_3Sc_2Si_3O_{12}$:Mn | 575, 680 |
| $Ca_2Si_5N_8:Eu^{2+}$ | 605 |
| $Sr_2Si_5N_8:Eu^{2+}$ | 620 |
| $Ba_2Si_5N_8:Eu^{2+}$ | 580 |
| $Ca_2Si_5N_8:Ce^{3+}$ | 470 |
| $Sr_2Si_5N_8:Ce^{3+}$ | 553 |
| $Ba_2Si_5N_8:Ce^{3+}$ | 451 |
| $CaSi_2O_2N_2:Eu^{2+}$ | 560 |
| $SrSi_2O_2N_2:Eu^{2+}$ | 530-570 |
| $BaSi_2O_2N_2:Eu^{2+}$ | 500 |
| $LaSr_2AlO_5:Ce^{3+}$ | 556 |
| La1-x$Sr_2-$x$Al_1-$xSix$O_5:Ce^{3+}$ | 533 (x = 0.8) |
| $Sr_3(AlO_4F)_{0.5}(SiO_5)_{0.5}:Ce^{3+}$ | 525 |
| $Sr_2Ba(AlO_4F)_{0.5}(SiO_5)_{0.5}:Ce^{3+}$ | 539 |
| GPT-4, 4k context length | |
| $Ca_2Si_5N_8:Eu^{2+}$ | 605 |
| $Sr_2Si_5N_8:Eu^{2+}$ | 620 |
| $Ba_2Si_5N_8:Eu^{2+}$ | 580 |
| $Ca_2Si_5N_8:Ce^{3+}$ | 470 |
| $Sr_2Si_5N_8:Ce^{3+}$ | 553 |
| $Ba_2Si_5N_8:Ce^{3+}$ | 451 |
| $CaSi_2O_2N_2:Eu^{2+}$ | 560 |
| $SrSi_2O_2N_2:Eu^{2+}$ | 530-570 |
| $BaSi_2O_2N_2:Eu^{2+}$ | 500 |
| $LaSr_2AlO_5:Ce^{3+}$ | 556 |
| $Sr_3(AlO_4F)_{0.5}(SiO_5)_{0.5}:Ce^{3+}$ | 525 |

| Chemical formula | Emission peak / nm (continued) |
| --- | --- |
| $Sr_2Ba(AlO_4F)_{0.5}(SiO_5)_{0.5}$:$Ce^{3+}$ | 539 |
| GPT-4, 6k context length | |
| No phosphors found (!) | |
| GPT-3.5, 2k context length | |
| $Y_{3-x}Ce_xAl_5O_{12}$:$Eu^{2+}$ | Not mentioned |
| GaN | Not mentioned |
| (Ga, In)N | Not mentioned |
| YAG:Ce | Not mentioned |
| $M_2SiO_4$:$Eu^{2+}$ | 500-600 |
| $Ba_2SiO_4$:$Eu^{2+}$ | 500 |
| $Sr_2SiO_4$:$Eu^{2+}$ | 575 |
| $BaSrSiO_4$:$Eu^{2+}$ | tunable |
| $M_2SiO_4$:$Ce^{3+}$ | 390 |
| $Ca_2SiO_4$:$Ce^{3+}$ | yellow |
| YAG:Ce | 540 |
| $Ca_3Sc_2Si_3O_{12}$:Ce | 505 |
| $Ca_3Sc_2Si_3O_{12}$:Ce, Mn | 575, 680 |
| $M_2Si_5N_8$:Ca | 605 |
| $M_2Si_5N_8$:Sr | 620 |
| $M_2Si_5N_8$:Ba | 580 |
| $MSi_2O_2N_2$:Ca | 560 |
| $MSi_2O_2N_2$:Sr | 530-570 |
| $MSi_2O_2N_2$:Ba | 500 |
| $LaSr_2AlO_5$:$Ce^{3+}$ | 556 |
| $Sr_3(AlO_4F)_{0.5}(SiO_5)_{0.5}$:$Ce^{3+}$ | 525 |
| $Sr_2Ba(AlO_4F)_{0.5}(SiO_5)_{0.5}$:$Ce^{3+}$ | 539 |

Supplementary Table 4: CGCNN model parameters and performance (full 10-fold "cross"-validation)

| CIF source | Unit cell | Optimizer | $R^2$ | MAE / eV |
|---|---|---|---|---|
| | | | 0.66 | 0.20 |
| | | | 0.70 | 0.19 |
| | | | 0.72 | 0.19 |
| | | | 0.71 | 0.19 |
| | | Adam | 0.68 | 0.20 |
| | | | 0.67 | 0.20 |
| | | | 0.39 | 0.26 |
| | | | 0.47 | 0.24 |
| | | | 0.69 | 0.20 |
| | Conventional cell | | 0.68 | 0.19 |
| | | | 0.64 | 0.22 |
| | | | 0.36 | 0.25 |
| | | | 0.74 | 0.19 |
| | | | 0.64 | 0.21 |
| | | SGD | 0.74 | 0.17 |
| | | | 0.69 | 0.19 |
| | | | 0.69 | 0.20 |
| | | | 0.67 | 0.20 |
| | | | 0.73 | 0.19 |
| | | | 0.40 | 0.25 |
| | | | 0.67 | 0.21 |
| | | | 0.67 | 0.20 |
| | | | 0.74 | 0.19 |
| | | | 0.73 | 0.20 |
| | | Adam | 0.73 | 0.19 |
| | | | 0.75 | 0.18 |
| | | | 0.63 | 0.21 |
| | | | 0.53 | 0.23 |
| | | | 0.73 | 0.19 |
| | | | 0.72 | 0.19 |
| ICSD | Primitive cell | | 0.59 | 0.21 |

SGD

| CIF source | Unit cell | Optimizer | $R^2$ | MAE / eV |
|---|---|---|---|---|
| | | | 0.75 | 0.19 |
| | | | 0.72 | 0.19 |
| | | | 0.67 | 0.21 |
| | | | 0.21 | 0.27 |
| | | | 0.65 | 0.20 |
| | | | 0.32 | 0.27 |
| | | | 0.69 | 0.20 |
| | | | 0.46 | 0.23 |
| | | | 0.65 | 0.20 |
| | ICSD original | Adam | 0.74 | 0.19 |
| | | | 0.12 | 0.27 |
| | | | 0.71 | 0.19 |
| | | | 0.75 | 0.18 |
| | | | 0.52 | 0.23 |
| | | | 0.73 | 0.18 |
| | | | 0.70 | 0.19 |
| | | | 0.75 | 0.18 |
| | | | 0.77 | 0.18 |
| | | | 0.74 | 0.17 |
| | | SGD | 0.70 | 0.19 |
| | | | 0.72 | 0.20 |
| | | | 0.53 | 0.23 |
| | | | 0.32 | 0.25 |
| | | | 0.46 | 0.25 |
| | | | 0.42 | 0.23 |
| | | | 0.46 | 0.25 |
| | | | 0.74 | 0.19 |
| | | | 0.60 | 0.21 |
| | | | 0.69 | 0.21 |
| Materials Project | Primitive | Adam | 0.72 | 0.17 |
| | | | 0.69 | 0.19 |
| | | | 0.68 | 0.20 |
| | | | 0.65 | 0.19 |
| | | | 0.73 | 0.18 |
| | | | 0.69 | 0.19 |

| CIF source | Unit cell | Optimizer | $R^2$ | MAE / eV |
|---|---|---|---|---|
| | | | 0.71 | 0.19 |
| | | | 0.67 | 0.19 |
| | | | 0.68 | 0.19 |
| | | | 0.66 | 0.19 |
| | | SGD | 0.71 | 0.18 |
| | | | 0.70 | 0.19 |
| | | | 0.65 | 0.20 |
| | | | 0.63 | 0.20 |
| | | | 0.60 | 0.21 |
| | | | 0.61 | 0.20 |
| | | | 0.51 | 0.24 |
| | | | 0.63 | 0.19 |
| | | | 0.58 | 0.20 |
| | | | 0.71 | 0.19 |

Supplementary Table 5: GPT-4 prompt (full)

**System**: You are a chemistry researcher.

**User**: A phosphor (such as $Y_3Al_5O_{12}$:$Eu^{2+}$) consists of a host lattice ($Y_3Al_5O_{12}$) doped with an activator ion ($Eu^{2+}$). Phosphors emit light in a spectrum. A phosphor's photoluminescence (PL) spectrum has an emission peak wavelength ($\lambda_{em}$), measured in nanometers (nm).
In addition to the emission peak, it also has an excitation peak ($\lambda_{ex}$) and an absorption peak, but they are irrelevant.
For example, $LiSrPO_4$:$Eu^{2+}$ has an emission peak at 445nm, whereas for $Sr_4Al_{14}O_{25}$: $Eu^{2+}$−$Dy^{3+}$, $\lambda_{em}$=490 nm.

**User**: Based on the following excerpt from a research article about phosphors, please create a table with two columns: 'chemical formula', and 'emission peak / nm'. Skip any entry if the emission peak is not mentioned in the text. Respond with nothing if no phosphor together with its emission peak is mentioned.
"The $Eu^{2+}$−$Mn^{2+}$ system is one of the most abundant systems for emission color adjustment in wLEDs phosphors. Liu et al. synthesized a novel blue to green phosphor $\gamma$-AlON:$Eu^{2+}$−$Mn^{2+}$. They found the $Eu^{2+}$ singly doped $\gamma$-AlON can emit a wide band centered at 470 nm corresponding to a blue color with an excitation band from 200 to 450 nm, and $Mn^{2+}$ singly-doped $\gamma$-AlON can produce a broad band peaking at 517 nm under 450 nm excitation."
| chemical formula | emission peak / nm |

**Assistant**:
| $\gamma$-AlON:$Eu^{2+}$ | 470 |
| $\gamma$-AlON:$Mn^{2+}$ | 517 |

**User**: Based on the following excerpt from a research review article about phosphors, please create a table with two columns: 'chemical formula', and 'emission peak / nm'. Skip any entry if the emission peak is not mentioned in the text. Respond with nothing if no phosphor together with its emission peak is mentioned.
{Text to be parsed}
| chemical formula | emission peak / nm |

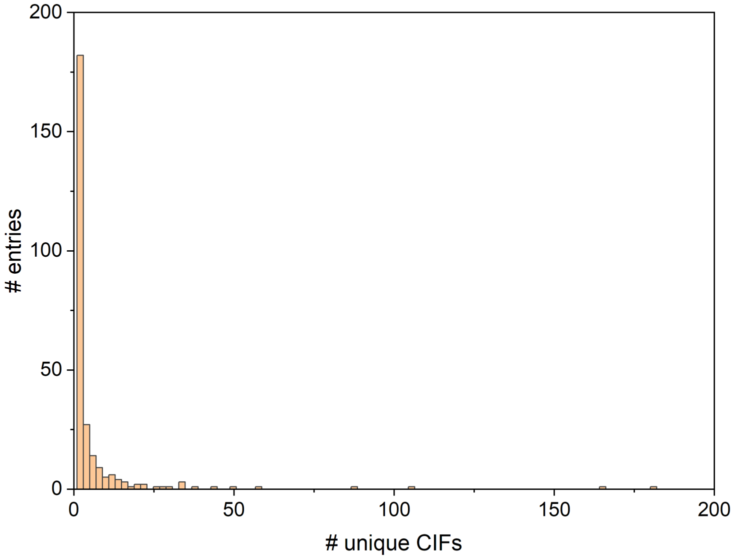


Supplementary Figure 1: Number of chemical formulas that found multiple matches in the ICSD.

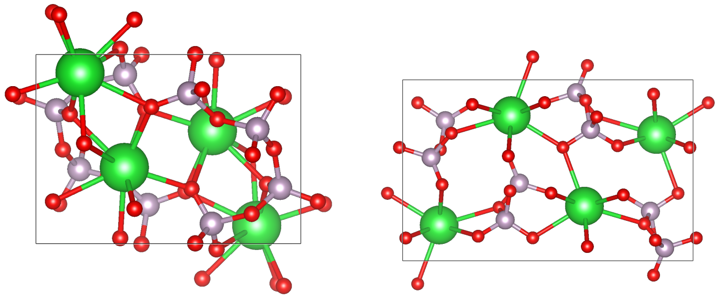

Supplementary Figure 2: (Rare) example of multiple ICSD matches that have actually different structures, $Ba(PO_3)_3$

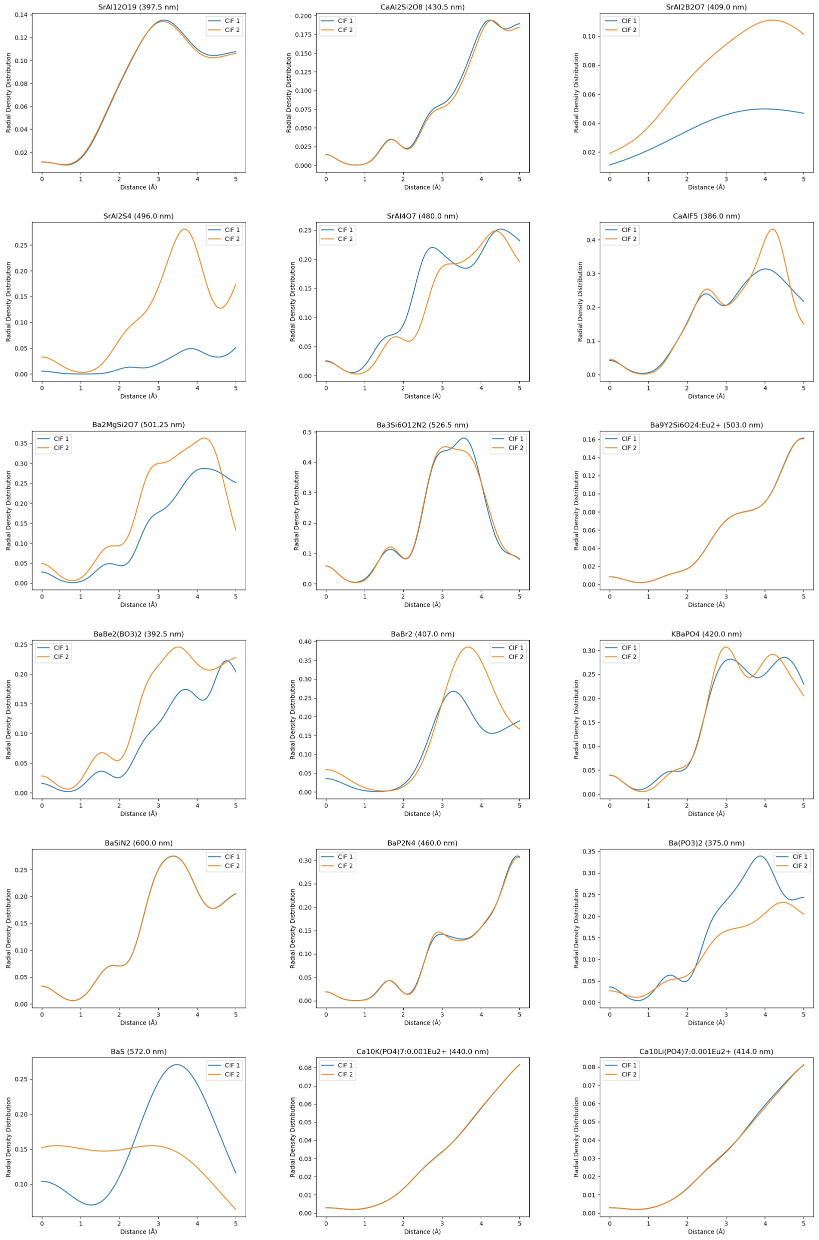


Supplementary Figure 3: Comparison of bond length distributions among multiple ICSD CIFs with identical chemical formulas, all cases with exactly 2 ICSD CIF matches. Most of them are simply duplicates.

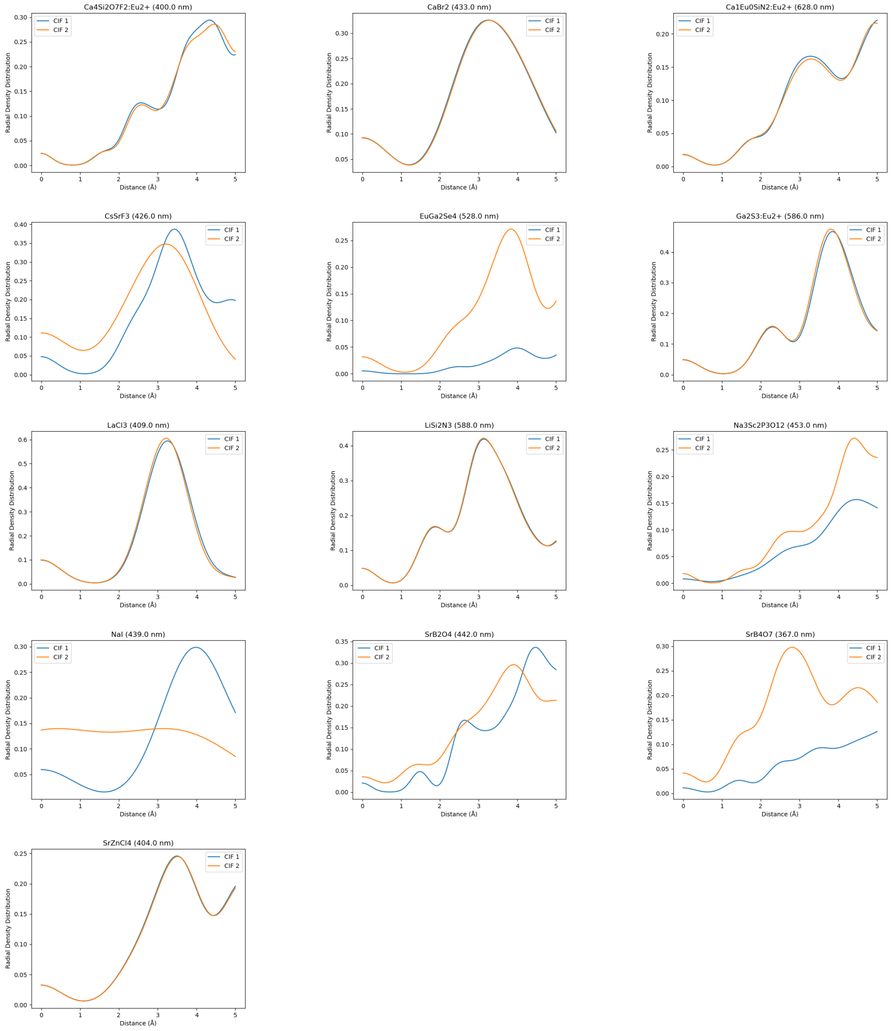


Supplementary Figure 4: Comparison of bond length distributions among multiple ICSD CIFs with identical chemical formulas (continued).

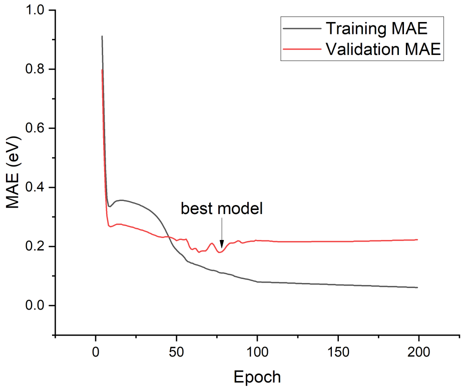


Supplementary Figure 5: Learning curve (and “early stopping”) for the CGCNN model trained on the ICSD dataset.

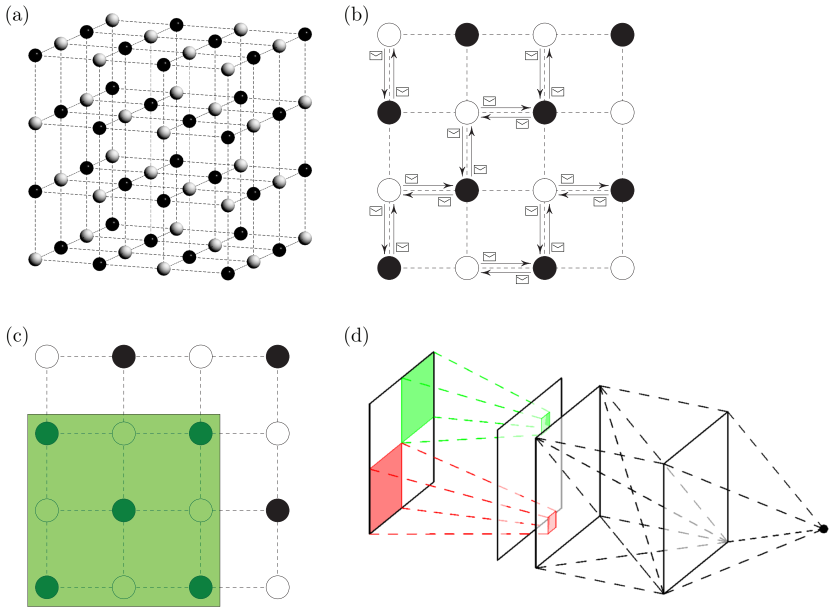


Supplementary Figure 6: CGCNN working principle. (a) Crystal structure. (b) Message passing. (c) Pooling. (d) Dense and readout.

# References


[1] Nathan C George, Kristin A Denault, and Ram Seshadri. Phosphors for solid-state white lighting. *Annual Review of Materials Research*, 43:481–501, 2013.

[2] John C Thomas, Anirudh Raju Natarajan, and Anton Van der Ven. Comparing crystal structures with symmetry and geometry. *npj Computational Materials*, 7(1):164, 2021.

[3] David C Lonie and Eva Zurek. Identifying duplicate crystal structures: Xtalcomp, an open-source solution. *Computer Physics Communications*, 183(3):690–697, 2012.

[4] Tian Xie and Jeffrey C Grossman. Crystal graph convolutional neural networks for an accurate and interpretable prediction of material properties. *Physical review letters*, 120(14):145301, 2018.

[5] P Dorenbos. Energy of the first 4f7→ 4f65d transition of eu2+ in inorganic compounds. *Journal of luminescence*, 104(4):239–260, 2003.

[6] Leland McInnes, John Healy, and James Melville. Umap: Uniform manifold approximation and projection for dimension reduction. *arXiv preprint arXiv:1802.03426*, 2018.
